# Supplementary material for: Smoothness of Directed Chain Stochastic Differential Equations
Source: arXiv:2202.09354 source file (2022-04-16)
Supplement: Supplementary file 1 [file appendix.tex]

\subsection{Maximum Likelihood Estimator of $u$}
\label{appen:mle_u}

By the fact of constant volatility in the directed chain model, the conditional log likelihood function \cite{feigin1976maximum} given observation $\mbX$ is 
\begin{equation}
\label{def:loglikelihood}
 l_u := \EE[-\log Z_t | \mcF^\mbX_T] = \EE\bigg[\int_0^t b(s, \mbX_s, \mbF_s)^T \ud \mbX_s  -\half\int_0^t |b(s, \mbX_s, \mbF_s)|^2 \ud s\bigg].
\end{equation}
This $l_u$ is quadratic in $u$ and can be maximized over $u$. We are hence able to derive a maximum likelihood estimator of $u$, that is
\begin{align}
\label{def:mle_u}
\widehat{u}_k = &\bigg[ \sum_{i=1}^{k-1}\int_0^T \bar{b}_{s, i}^2 \ud s + \EE\big[\int_0^T \bar{b}_{s, k}^2 \ud s | \mcF^\mbX_T\big] \bigg]^{-1} \times \nonumber \\
& \bigg\{ \sum_{i=1}^{k-1}\int_0^T\bar{b}_{s, i}\big( \ud X_{s, i} - \int_\RR \tilb(s, X_{s, i}, y) \mu_s(\ud y)\ud s \big) + \nonumber\\
&\qquad \EE\big[\int_0^T\bar{b}_{s, k}\big( \ud X_{s, k} - \int_\RR \tilb(s, X_{s, k}, y) \mu_s(\ud y)\ud s\big)| \mcF^\mbX_T\big]\bigg\},
\end{align}
where $\bar{b}_{s, i} = \tilb(s, X_{s, i}, X_{s, i+1}) - \int_\RR \tilb(s, X_{s,i}, y) \mu_s(\ud y)$.

Notice that in this \eqref{def:mle_u}, we use particle $X_{1}, \dots, X_{k+1}$ but remove the randomization of $X_{k+1}$ to get the estimation. We can also use only $X_{1}, \dots, X_{k}$ to get the MLE when $k\ge 2$, the only difference is that the expectation terms disappear in both numerator and denominator. When the observation is independently identically distributed (\textit{i.i.d}), it is straightforward that the maximum likelihood estimator is converging to the true value and follows asymptotic central limit theorem. But in this directed chain model, observations $X_{\cdot, 1}, \dots, X_{\cdot, k}$ are correlated. This structure makes the convergence and speed of convergence nontrivial. Fortunately, when $k\to\infty$, we can get a limit of $\widehat{\mu}_k$ by the ergodic theorem, which can be shown to be the true value of $u$.

\begin{prop} \label{prop:mle_u}
Assume $$\int_0^T |\bar{b}_{i, s}|^2 \ud s >0 \text{ a.s.},$$
we let $n\to\infty$, the maximum likelihood estimator $\widehat{u}_k$ converges almost surely to the true value $u$, that is,
\begin{equation}
\label{def:limit_mle_u}
	\lim_{k\to\infty} \widehat{u}_k = \frac{\EE\big[\int_0^T \bar{b}_{s, 1} \big(\ud X_{s, 1} - \int_\RR \tilb(s, X_{s, 1}, y)\mu_s(\ud y)\ud s\big)\big]}{\EE\big[\int_0^T |\bar{b}_{s, 1}|^2 \ud s \big]} \equiv u.
\end{equation}
\end{prop}
\begin{proof}
The limit exists $\PP$ almost surely by the Chacon-Ornstein theorem and the second equality can be verified by rewriting the dynamics of $X$. We first proof the second equality. We rewrite \eqref{def:sde_X} as
$$\ud X_{s, 1} = (u \bar{b}_{s, 1} + \int_\RR \tilb(s, X_{s, 1}, y) \mu_s(\ud y)) \ud s + \ud B_s$$
by the definition of $b$ in \eqref{def:b} and $\bar{b}$. The numerator becomes 
$$u\cdot \EE\big[\int_0^T  |\bar{b}_{s, 1}|^2 \ud s\big] + \EE\big[\int_0^T \bar{b}_{s, 1} \ud B_s\big]$$ 
where the second term is $0$ because of the integrability $ \EE[\int_0^T  |\bar{b}_{s, 1}|^2 \ud s]<\infty$. We have proved the ratio is $u$. 

We let $n\to\infty$ and denote $\tau: (X_{\cdot, i}, X_{\cdot,i+1}, \dots) \to (X_{\cdot,i+1}, X_{\cdot,i+2}, \dots)$ the shifting operator. Define $\tau f(X_{\cdot, i}, X_{\cdot, i+1}, \dots) := f(\tau(X_{\cdot, i}, X_{\cdot,i+1}, \dots))$ for every bounded measurable function and $\tau^k := \tau \circ \tau^{k-1}$ for $k\ge 1$. Due to the special structure of directed chain model, $\tau$ is a measure preserving map, i.e. $\Law(X_{\cdot, 1}, X_{\cdot, 2}, \dots, X_{\cdot, j})= \Law(X_{\cdot, i}, X_{\cdot, i+1}, \dots, X_{\cdot, i+j})$ $\forall i=1, 2, \dots$. 

In order to apply Chacon-Ornstein theorem, we need to show that $\tau$ is conservative and ergodic \cite[Appendix Theorem 5.2]{revuz2013continuous}.
Let $f$ be a positive almost surely and integrable function, then we have $\forall k\ge 0$, $\tau^k f > 0$ a.s.. Define $\sigma$ field $\mcG_n := \sigma ((X_{0, i}, B_{\cdot, i}))$ generated by $X_{0, i}$ and the corresponding Brownian path and the tail sigma field $\mcG_{\infty}:= \wedge_{m\ge 1}\vee_{n\ge m} \mcG_n$. 
It is immediate that $\mcG_n$'s are independent and the event
$$\{\sum_{k\ge 0} \tau^k f =\infty\} \in\mcG_{\infty},$$
hence $\PP(\sum_{k\ge 0} \tau^k f =\infty) = 0 \text{ or }1$ by Kolmogorov zero-one law. 
\begin{align}
\PP(\sum_{k\ge 0} \tau^k f < \infty) &= \PP(\lim_{m\to \infty}\sum_{k\ge m} \tau^k f =0) \nonumber \\
&= \PP\big(\bigcap_{\epsilon>0} \{\lim_{m\to \infty}\sum_{k\ge m} \tau^k f < \epsilon\}\big) \nonumber \\
&= \lim_{\epsilon\to 0} \lim_{m\to\infty}\PP\big(\{\sum_{k\ge m} \tau^k f < \epsilon\}\big) \nonumber \\
&\le \lim_{\epsilon\to 0} \lim_{m\to\infty} \PP(\tau^m f < \epsilon) \nonumber \\
&\overset{(i)}{=} \lim_{\epsilon\to 0} \PP(f < \epsilon) = 0,
\end{align}
where we use the measure preserving property in the equality (i) and positivity of $f$ to derive the limit. Then we get the result $\PP(\sum_{k\ge 0} \tau^k f =\infty)=1$ and hence $\tau$ is conservative. Replace $f$ to be an element in $L_+^1$ such that $f\not\equiv 0$, it follows that $\PP(\sum_{k\ge 0} \tau^k f =\infty)=1$ since $\lim_{\epsilon\to 0}\PP(f<\epsilon) < 1$ and hence $\PP(\sum_{k\ge 0} \tau^k f <\infty)=0$ again by zero one law. We have $\tau$ is ergodic \cite{neveu1979}. Let $f:= \int_0^T |\bar{b}_{s, 1}|^2 \ud s$ and $g:= \int_0^T\bar{b}_{s, 1}(\ud X_{s, 1} - \int_\RR\tilb(s, X_{s, 1}, y)\ud y \ud s).$
By the Chacon-Ornstein theorem, the limit is
$$\lim_{k\to\infty}\widehat{u}_k = \frac{\EE[g]}{\EE[f]}$$ and equals to the $u$ in \eqref{def:limit_mle_u}.
\end{proof}

Given the convergence result, a natural question to ask next is how fast does it converge.
By \cite[Theorem 3]{denker1986uniform}, we are also able to derive a central limit theorem (CLT) for the MLE $\widehat{u}_T$.
\begin{prop}
\label{prop:clt_u}
Denote $\sigma_k^2 := \sum_{i=1}^{k-1}\int_0^T \bar{b}_{s, i}^2 \ud s$ and $\bar{\sigma}_k^2 = \EE[\sigma_k^2]$, then we have 
\begin{equation}
	\bar{\sigma}_{k} \cdot (\widehat{u}_k-u) \overset{D}{\longrightarrow} \mcN(0, 1).
\end{equation}
\end{prop}
\begin{proof}
	Denote $s_k :=  \sum_{i=1}^{k-1}\int_0^T\bar{b}_{s, i}\big( \ud X_{s, i} - \int_\RR \tilb(s, X_{s, i}, y) \mu_s(\ud y)\ud s \big)$. By rewriting $\ud X_{s, i}$, we have
	$$s_k - u\cdot\sigma^2_k = \sum_{i=1}^{k-1}\int_0^T\bar{b}_{s, i} \ud B_{s, i}.$$
	As we have proved in Proposition \ref{prop:mle_u}, $\sigma_k\overset{k\to\infty}{\longrightarrow} \infty$ $a.s.$ (so as $\bar{\sigma}_k$) and hence 
	$$\lim_{k\to\infty} \big(\bar{\sigma}_{k} \cdot (\widehat{u}_k-u) - \bar{\sigma}_{k}(\frac{s_k}{\sigma^2_k}-u)\big)=0, \quad a.s.$$
	where we use the result that $\lim_{k\to\infty}\bar{\sigma}^2_{k}/\sigma^2_k = 1$ by Proposition \ref{prop:mle_u}.
	The goal is to show $\bar{\sigma}_k(s_k/\sigma^2_k-u)$ converges to a standard normal random variable weakly which is equivalent to prove $(s_k - u \sigma^2_k)/\bar{\sigma}_k$ converges to standard normal distribution. To simplify notation, we let $S_k = s_k-u\cdot\sigma^2_k$. Note that the strong mixing condition is satisfied automatically by the strictly stationarity of $\{\int_0^T \bar{b}_{s,i}\ud B_{s,i}\}_{i\ge 1}$ sequence. It remains to show the uniform integrability of $\{\bar{\sigma}_k^{-2}S_k^2\}_{k\ge 1}$ by \cite[Theorem 3]{denker1986uniform}. Note that $\bar{\sigma}_k^2 = (k-1) \bar{\sigma}_1^2$
	\begin{align}
	\label{def:ui}
	\EE\bigg[ \frac{S^2_k}{\bar{\sigma}_k^2} \cdot \I_{\{S^2_k/\bar{\sigma}_k^2>\lambda\}} \bigg] &= \frac{1}{\bar{\sigma}_k^2} \EE\big[ \big( S_k  \I_{\{S^2_k/\bar{\sigma}_k^2>\lambda\}}\big)^2\big] \nonumber\\
	&= \frac{1}{\bar{\sigma}_k^2} \sum_{i=1}^{k-1} \EE\big[ \int_{0}^T \bar{b}^2_{s, i}\I_{\{S^2_k/\bar{\sigma}_k^2>\lambda\}} \ud s\big] \nonumber \\
	&=  \frac{k-1}{\bar{\sigma}_k^2} \EE\big[ \int_{0}^T \bar{b}^2_{s, 1} \ud s\cdot \I_{\{S^2_k/\bar{\sigma}_k^2>\lambda\}}\big] \nonumber \\
	&= \frac{1}{\bar{\sigma}_1^2}\EE\big[ \int_{0}^T \bar{b}^2_{s, 1} \ud s\cdot \I_{\{S^2_k/\bar{\sigma}_k^2>\lambda\}}\big].
	\end{align}
	Since a single random variable $ \int_{0}^T \bar{b}^2_{s, 1} \ud s$ is uniformly integrable, and 
	$$\sup_{k\ge 1}\PP(S^2_k/\bar{\sigma}_k^2>\lambda) <\sup_{k\ge 1} \frac{1}{\lambda}\EE[S^2_k/\bar{\sigma}_k^2] = \frac{1}{\lambda}.$$
	Take supremum on both sides of \eqref{def:ui}, we get $\forall\epsilon>0$, 
	$$\sup_{k\ge 1}\EE\bigg[ \frac{S^2_k}{\bar{\sigma}_k^2} \cdot \I_{\{S^2_k/\bar{\sigma}_k^2>\lambda\}} \bigg] < \epsilon $$
	for sufficiently large $\lambda$, and hence $\{\bar{\sigma}_k^{-2}S_k^2\}_{k\ge 1}$ is uniformly integrable.
\end{proof}
